# Supplementary material for: Lessons from the Vacuum Structure of 4d N=2 Supergravity
Source: arXiv:1207.3830 source file (2013-03-13)
Supplement: Supplementary file 1 [file appN1.tex]

%%%%%%%%%%%%%%%%%%%%%%%%%%%%%%%%%%%%%%%%
\chapter{Calculations with NS5-branes}
\label{app:ns5calc}\label{ap:ns5calc}
%%%%%%%%%%%%%%%%%%%%%%%%%%%%%%%%%%%%%%%%
In this appendix we give some details of the calculations which have
been used in chapter~\ref{chapter::ns5}.

We want to calculate the derivatives and inverses for the K\"ahler potentials~\eqref{KIIBLVS}
\begin{align}\label{ap:kahlerpot}
\mathcal  K_0 &= - \ln (-i (\tau-\bar \tau)) - 2 \ln \left(\mathcal V + \frac {\hat \xi}2\right),\\
\mathcal   K_{\rm NS5} &= B \mathcal V^n \exp\big(- \mathcal V \tau_2^2)\,,
\end{align}
where we use
\begin{align}
\begin{split}
  \tau &= l + i {\rm e}^{\phi},\\ \tau_2 &= \text {Im}\  \tau\,,\\
 6 \mathcal V &= \mathcal K_{ijk} t^it^jt^k = \mathcal K_{ij}t^it^j = \mathcal K_i t^i\,,\\
 \hat \xi &= \xi (\text {Im} \, \tau)^{3/2}.
\end{split}
\end{align}
We introduce $\mathcal K^{ij}$ as the inverse of $\mathcal K_{ij}$, and denote $\mathcal A := \mathcal V + \hat \xi
/2$. We first consider the case where $G^a = 0$. From $T_i = \tau_i + ib_i$ (equation~\eqref{chiral-fields1} for $G^a=0$) we find
\begin{align}
  \frac {\partial t^j}{\partial T_i} = \frac 14 \mathcal K^{ij},\quad \frac {\partial \mathcal V}{\partial T_i} = \frac 18 t^i.
\end{align}
We can then calculate
\begin{align}
\begin{split}
\mathcal K^0_{T_i} &= - \frac 1 4 \frac {t^i}{\mathcal A},\quad \mathcal K^0_\tau = i \tau_2^{-1} \left(\frac {3 \hat \xi}{4\mathcal A} + \frac 12 \right)\,,\\
\mathcal K^0_{T_i\bar T_j} &= \frac {G^{ij}}{\mathcal A^2},\quad
G^{ij} = - \frac 1 {16} \mathcal A \mathcal K^{ij} + \frac 1 {32} t^it^j\,,\\
\mathcal K^0_{i \bar \tau} &= \frac {3i}{32\mathcal A^2} \tau_2^{-1} \hat \xi t^i\,,\\
\mathcal K^0_{\tau \bar \tau} &= \frac 1 {16} \tau_2^{-2} \mathcal A^{-2} (4 \mathcal V^2 + \mathcal V \hat
\xi + 4 \hat \xi^2)\,.
\end{split}
\end{align}
This can be inverted to give
\begin{align}
\begin{split}
\mathcal K_0^{\tau \bar \tau} &= \frac{4\mathcal V - \hat \xi}{\mathcal V - \hat \xi} \tau_2^2\,,\\
\mathcal K_0^{i\bar \tau} &= -\frac {3i \hat \xi}{\mathcal V - \hat \xi} \tau_2 \mathcal K_i\,,\\
\mathcal K_0^{i\bar \jmath} &= -8 (2\mathcal V + \hat \xi) \mathcal K_{ij} + \frac {4\mathcal V-\hat \xi}{\mathcal
V-\hat \xi} \mathcal K_i\mathcal K_j\,.
\end{split}
\end{align}
We then find a familiar result, which leads directly to~\eqref{VLVS}:
\begin{align}\label{pot:bbhl}
\mathcal   K_0^{\alpha \bar \beta}\mathcal  K^0_{\alpha} \mathcal K^0_{\bar \beta} = 3 + \frac { 3\hat \xi (\mathcal V^2 + 7
  \mathcal V \hat \xi + \hat \xi^2)}{(\mathcal V - \hat \xi)(2 \mathcal V + \hat\xi)^2}\,.
\end{align}
For the NS5--brane contribution we obtain (we write $\mathcal K_5 = \mathcal K^5 = \mathcal K_{\rm NS5}$)
\begin{align}
\begin{split}
\mathcal K^5_{\tau \bar \tau} &= -\frac 14 \mathcal K_5 \mathcal V ((\tau-\bar \tau)^2 \mathcal V + 2)\,,\\
\mathcal K^5_{i \bar \tau} &= \frac i 8 B\exp(-\mathcal V\tau_2^2) \mathcal V^n (-\mathcal V \tau_2 + n + 1) \tau_2 t^i\,,\\
\mathcal K^5_{i \bar \jmath} &= \frac 1 {64} B t^it^j \mathcal V^{n-2} \left(\mathcal V^2 \tau_2^4
-\mathcal V 2 n \tau_2^2 + (n-1)n\right)\exp(-\mathcal V \tau_2^2)\,.
\end{split}
\end{align}
We are interested in the leading term in the potential, so we want to investigate the powers of the
volume. If we denote volume powers with $[\cdot]$, then
\begin{align}
  [\mathcal V] = 1\,, \quad [\mathcal K_{ijk}]=0\,, \quad [t^i]=\frac 13\,, \quad [\mathcal K_{ij}]=\frac 13\,.
\end{align}
All the one--instanton terms are multiplied by $\exp (-\mathcal V \tau_2^2)$. To determine the leading term, we have to find the highest power of the volume $\mathcal V$ in the polynomial which appears in front of this exponent. Therefore, we do not include the factor $\exp(-\mathcal V \tau_2^2)$ in the counting, or equivalently we put $[\exp(-\mathcal V \tau_2^2)]=0$.

The various terms have the following leading volume dependencies:
\begin{align}
  [\mathcal K_0^{i\bar \jmath}] &= 4/3 &&& [\mathcal K^5_{i    \bar \jmath}] &= n+2/3  &&& [\mathcal K_0^{i \bar \jmath}\mathcal  K^5_{\bar \jmath k   }\mathcal  K_0^{\bar k    l}] &= n+10/3\nonumber\\
  [\mathcal K_0^{i\bar \tau}] &= -1/3  &&& [\mathcal K^5_{i    \bar \tau  }] &= n+4/3  &&& [\mathcal K_0^{i \bar \tau} \mathcal   K^5_{\bar \tau   k   } \mathcal K_0^{\bar k    l}] &= n+7/3\\
  [\mathcal K_0^{\tau\bar \tau}] &= 0  &&& [\mathcal K^5_{\tau \bar \tau  }] &= n+2    &&& [\mathcal K_0^{i \bar \tau}\mathcal  K^5_{\bar \tau   \tau}\mathcal  K_0^{\bar \tau l}] &= n+4/3\,.\nonumber
\end{align}
The leading contribution is given by (we use $\simeq$ here to denote equality up to subleading terms)
\begin{align}
\mathcal K_5^{i\bar \jmath} =\mathcal  K_0^{i\bar \alpha} \mathcal K^5_{\bar \alpha \beta}\mathcal K_0^{\beta \bar \jmath} \simeq \mathcal K_0^{i\bar l}\mathcal K^5_{\bar l k}\mathcal K_0^{k \bar \jmath} \simeq B  \mathcal V^{n+2} g_s^{-4}
\exp(-\mathcal V/g_s^2)\mathcal K_i \mathcal K_j\,.
\end{align}
We remind that $\mathcal K_5^{i\bar \jmath}$ is the inverse of $\mathcal K_{5,\alpha
  \bar \beta}$ in the directions of the K\"ahler moduli. In the potential we find then $[\mathcal K_5^{i\bar \jmath} |\partial_i \mathcal K_0|^2] = (n+10/3) - 2/3 - 2/3 =
n+2$. The other term is $[\mathcal K_0^{ij} \partial_i \mathcal K^5 \partial_{\bar \jmath} \mathcal K_0] = 4/3 + (n+1/3) - 2/3
= n+1$, which is subleading with respect to the terms above. Then the leading contribution to the scalar potential is given by
\begin{align}\label{ap:potfinal}
  \begin{split}
  V &\simeq -{\rm e}^{\mathcal K_0}\mathcal K_{{\rm NS5}}^{i\bar \jmath}\,|\partial_i \mathcal K_0|^2 |W_0|^2\\
  &= -\frac 9 8 B \mathcal V^n g_s^{-3} |W_0|^2 \exp (-\mathcal V/ g_s^2)\,.
  \end{split}
\end{align}

Let us now consider the effects of non-zero $G^a$, to clarify the statements made after equation~\eqref{ns5inverse}. From the definition~\eqref{chiral-fields1}
\begin{align}
  T_i =  \tau_i + ib_i + \frac{i}{\tau-\bar\tau} \, \mathcal K_{iab}G^a (G-\bar G)^c\,,
\end{align}
we find that
\begin{align}
  \frac {\partial t^j}{\partial T_i} = \frac 14 \mathcal K^{ij}\,,\quad
  \frac {\partial{t^i}}{\partial{G^a}} = \frac 1 4 \mathcal K^{i j} \mathcal K_{jab}b^b\,,\quad
  \frac {\partial{t^i}}{\partial \tau} = \frac i 2 \mathcal K_{iab}b^ab^b\,,
\end{align}
and hence
\begin{align}
  \frac {\partial \mathcal V}{\partial T_i} = \frac 18 t^i\,,\quad
  \frac {\partial \mathcal V}{\partial{G^a}} = \frac 12 t^j \mathcal K_{jac}b^c = \frac 12 \mathcal K_{ac}b^c\,,\quad
   \frac {\partial \mathcal V}{\partial \tau} = \frac i 4 t^j \mathcal K_{jab}b^ab^b = \frac i 4 \mathcal K_{ab}b^ab^b\,.
\end{align}
In the last two expressions the factor $t^j$ is bound with the factor $\mathcal K_{jac}$ and cannot combine with a $\mathcal K_j$ to
form a power of the volume. 

The expression for~\eqref{ns5inverse} also contains inverse metrics. If we use the expressions
for the tree--level K\"ahler metric in~\cite{Grimm:2004uq}, we can explicitly determine the volume
dependence, and we find
\begin{align}
\begin{split}
\mathcal   K_0^{ia}\mathcal K^5_{ab}\mathcal K_0^{bj} t^it^j &\sim \mathcal V^{n+2}\,,\\
\mathcal   K_0^{ik}\mathcal K^5_{kl}\mathcal K_0^{lj} t^it^j &\sim \mathcal V^{n+4}\,,\\
\mathcal   K_0^{ia}\mathcal K^5_{ak}\mathcal K_0^{kj} t^it^j &\sim
\mathcal V^{n+3}\,,
\end{split}
\end{align}
and the leading term does not contain the fields $G^a$. We do not know if this property holds when
we include quantum corrections to the K\"ahler potential, but as quantum corrections are expected
to be subleading in the volume, we expect this to be the case.

%%%%%%%%%%%%%%%%%%%%%%%%%%%%%%%%%%%%%%%%%%%%%%%%%
\section[\protect{Potentials in $\superN=2$}]{\protect{Potentials in $\mathbf{\superN=2}$}}\label{ap:n2}
%%%%%%%%%%%%%%%%%%%%%%%%%%%%%%%%%%%%%%%%%%%%%%%%%

In this appendix we give some more details of the calculation in the $N=2$ setting. This
appendix derives a general form of the scalar potential. The next appendix specializes this to the
UHM and the Przanowski metric.

We use the formalism from~\cite{deWit:2001bk} with the vector prepotential
\begin{align}\label{prepot-pert}
  F = \frac 1 {3!}  \frac{\mathcal K_{ijk} X^iX^jX^k}{X^0} + \frac {i}{2} \zeta(3)\chi(CY)
  X^0X^0\,.
\end{align}
From the prepotential we define
\begin{align}
\begin{split}
N_{IJ} &= -i F_{IJ} + i\bar F_{IJ} = 2 {\rm Im} \, F_{IJ},\\
\mathcal M_{IJ} &= \frac 1 {[N_{MN}X^M\bar X^N]^2} \left[ N_{IJ} N_{KL} - N_{IK} N_{JL} \right]
\bar X^K X^L\,,
\end{split}
\end{align}
and then the scalar potential is given by
\begin{align}
V =&-4 g^2 \left[2 G_{\alpha \bar \beta} k^{\alpha}_I k^{\beta}_J + 3 \vec \mu_I \cdot \vec
\mu_J\right] \frac {X^I \bar X^J}{N_{MN} X^M \bar X^N} \\ &- g^2 N_{MN} X^M \bar X^N \mathcal
M_{IJ} \left[4 N^{IK}N^{JL} \vec \mu_L \cdot \vec \mu_L - \frac {f_{KL}^I X^K \bar X^L}{N_{PQ} X^P
\bar X^Q} \frac {f_{MN}^J X^M \bar X^N}{N_{PQ} X^P \bar X^Q}\right],\nonumber
\end{align}
where $g$ is an overall factor to make the terms which are a result of the gauging more explicit in the Lagrangian; we put $g=1$ from now on. In general, each vector field in the vector multiplets can be used to gauge one of the $h^{1,1}+1$ different killing vectors $k^I$. In our setting, there is only one isometry $k$, which we gauge by the graviphoton. The index $I$
therefore only attains the value $0$. If we use $\vec \mu_I = \delta_I^0 \vec \mu$ we obtain
\begin{align*}
V =&- \frac{4}{N_{MN} X^M \bar X^N } \Big( \left[2 G_{\alpha \bar \beta} k^{\alpha} k^{\beta} +
3 \vec \mu ^2\right] X^0 \bar X^0 + ( N_{KL} N^{00} - \delta_K^0 \delta_L^0) \bar X^K X^L  \vec
\mu^2 \Big),
\end{align*}
and the term depending on $f_{KL}^I$ is zero for abelian gaugings. We now use the prepotential
\begin{align}
F = \frac 1 {3!} \mathcal K_{ijk} \frac {X^iX^jX^k}{X^0} + \frac 12 e X^0 X^0\,,
\end{align}
where $e = \frac i2 \zeta(3) \chi(CY)$ is purely imaginary. Using $X^i/X^0 =
z^i = b^i + i t^i$, we find
\begin{align}
F_{00} &= \frac 13 \mathcal K_{ijk} z^iz^jz^k + e & {\rm Im}\, F_{00} &= \mathcal K_{ijk} b^ib^jt^k - \frac 13 \mathcal K_{ijk}
t^it^jt^k\nonumber\\
 F_{0i} &= -\frac 12 \mathcal K_{ijk} z^jz^k & {\rm Im}\,  F_{0i} &= -\mathcal K_{ijk} b^jt^k\\
 F_{ij} &=  \mathcal K_{ijk} z^k & {\rm Im}\,  F_{ij} &=  \mathcal
 K_{ijk} t^k\,.\nonumber
\end{align}
Using the abbreviations $\mathcal K_{ij} = \mathcal K_{ijk} t^k, \mathcal K_i = \mathcal K_{ij}t^j, 6 \mathcal V = \mathcal K_{ijk}t^it^jt^k$ we
find
\begin{align}%\label{N-cubic-and-loop}
N_{00} &= 2 \mathcal K_{ij} b^ib^j -4\mathcal V' & N^{00} &= \frac {-1}  {4\mathcal V'}\nonumber
\\
N_{0i} &= -2 \mathcal K_{ij} b^j & N^{0i} &= \frac {-b^i} {4\mathcal V'}\\
N_{ij} &= 2\mathcal K_{ij} & N^{ij} &=  \frac{-b^ib^j}{4\mathcal V'} + \frac 12 d^{ij}\nonumber \\
{\rm e}^{-K} &\equiv N_{IJ}X^I \bar X^J = (8 \mathcal V + 2 e) X^0 \bar X^0 \,,\nonumber
\end{align}
where we have written $\mathcal V' := \mathcal V - \frac 12 e$. For the scalar potential we then finally find equation~\eqref{VUHM}
\begin{align}\label{V-cubic}
V&=- \frac{4}{8 \mathcal V + 2 e} \left( \left[2 G_{\alpha \bar \beta} k^{\alpha}
k^{\beta} + 3 \vec \mu ^2\right]  + ( 8 \mathcal V' \frac {-1} {4\mathcal V'} - 1) \vec \mu^2 \right), \nonumber\\
&= \frac{2}{4\mathcal V + e} \left[ -2 G_{\alpha \bar \beta} k^\alpha k^\beta \right].
\end{align}
The scalar potential is positive definite.

%%% Local Variables: 
%%% mode: latex
%%% TeX-master: "../thesis"
%%% End: 
