# Supplementary material for: Lessons from the Vacuum Structure of 4d N=2 Supergravity
Source: arXiv:1207.3830 source file (2013-03-13)
Supplement: Supplementary file 2 [file appPrzanowski.tex]

%%%%%%%%%%%%%%%%%%%%%%%%%%%%%%%%%%
\chapter{The Przanowski metric}
%%%%%%%%%%%%%%%%%%%%%%%%%%%%%%%%%%
\label{app:przanowski}

In this appendix we repeat some of the results of~\cite{Przanowski:1991ru,Alexandrov:2006hx}, which are used to determine the NS5--brane one--instanton corrected $N=2$ moduli space in section 3.2.

In \cite{Przanowski:1991ru}, it has been shown that a four-dimensional quaternionic-K\"ahler manifold $M$
can be described in terms of a partial differential equation for a single, real function. Locally, the metric takes the form
\begin{align}\label{eq:prmetric}
g &= g_{\alpha \bar \beta} (dz^\alpha \otimes dz^{\bar \beta} +
dz^{\bar \beta} \otimes dz^{\alpha})\\
&= g_{1\b1} dz^1 dz^\be + g_{1\b2} dz^1 dz^\bt + g_{2 \be} dz^2 dz^\be + g_{2 \bt} dz^2dz^\bt +
c.c.\,,\nonumber
\end{align}
where indices $\alpha,\beta,\bar \alpha,\bar \beta = 1,2$, and we have used the usual convention of
complex conjugation $z^{\bar \alpha} := \overline {z^\alpha}$. The Hermicity of this metric is
encoded in the requirement $\overline {g_{\alpha \bar \beta}} = g_{\beta \bar \alpha}$. The
elements $g_{\alpha \bar \beta}$ are now defined in terms of a real function $h =
h(z^\alpha,z^{\bar \alpha})$ via
\begin{align}\label{eq:prmetric2}
g_{\alpha \beta} = 2 \left(h_{\alpha \bar \beta} + 2 \delta_{\alpha}^2 \delta_{\bar \beta}^2 {\rm e}^h \right),
\end{align}
where the subscript $\alpha$ on $h_{\alpha}$ indicates differentiation of the function with respect
to $z^\alpha$. We have changed the sign of our defining function $h$ with respect to the
original function $u$ used by Przanowski, as it offers a slightly more convenient form to work
with.

The differential equation which determines the function $h$ is the non--linear partial differential
equation
\begin{align}\label{eq:prz}
h_{1\b1} h_{2\bt} - h_{1\bt} h_{\be2} + (2 h_{1\be} - h_1 h_{\be}) {\rm e}^h = 0\,.
\end{align}

\section{Solutions to the master equation} The equation~\eqref{eq:prz}
is a difficult partial differential equation. There have been various approaches in the literature
which found exact and approximate solutions to the master equation. By imposing
additional symmetries on the manifold $M$, one can simplify the master equation. Imposing one
isometry reduces this equation to the Toda equation~\cite{Przanowski:1991ru}. Upon imposing two commuting isometries one
obtains the Calderbank-Pedersen metrics~\cite{calderbank:2001uz}.

In~\cite{Alexandrov:2006hx}, solutions to the master equation where obtained which corresponded to
NS5--brane instantons. The relation between the complex coordinates and the real coordinates is
given by
\begin{align}
  z^1 = \frac 12 (u+i\sigma)\,,\quad z^2 = \frac 12 (\chi + i\varphi)\,, \quad u \equiv r - \frac 12 \chi^2 +
  c \log (r+c)\,.
\end{align}
The leading term of the one--instanton contribution is captured by
\begin{align}\label{equation:h}
\begin{split}
  h &= h_0 + \Lambda,\quad h_0 = \log (r+c) - 2 \log r\,,\\
  \Lambda &= C r^{-2-c} \cos(\sigma) \exp\left[-r + \frac 12
    \chi^2\right].
\end{split}
\end{align}
{}From the metric we only need the length of the Killing vector $k = \partial_\varphi$, which can be found from~\eqref{eq:prmetric},~\eqref{eq:prmetric2} and~\eqref{equation:h} and is given by
\begin{align*}
  -G_{\alpha \beta} k^\alpha k^\beta = \frac { 4((r+2c)^2 + (r+c)\chi^2)}{r^2(r+2c)} + 16 C r^{-2-c}
  (2\chi^2-1)
  \exp(-c-r-\chi^2/2)\,.
\end{align*}
Inserting this into~\eqref{V-cubic} yields~\eqref{VUHM}.

\section{Moment maps}
Although the moment maps are not present in the scalar potential, we include their calculation for
completeness. We follow the conventions on quaternionic-K\"ahler geometry from~\cite{Davidse:2005ef}.

We want to find vielbeins $a, b$ for the metric~\eqref{eq:prmetric} such that
\begin{align}
a \otimes \bar a + b \otimes \bar b + c.c. = {\rm ds}^2\,.
\end{align}
Using the Ansatz $a = \alpha {\rm d}z^1 + \beta {\rm d}z^2, b = \gamma {\rm d}z^1 + \delta {\rm d}z^2$ we find
\begin{align}
\begin{split}
a &=\sqrt{2 h_{1\b1}}\, {\rm d}z^1 + \sqrt {2} \frac{ h_{\be2}}{\sqrt{h_{1\b1}}}\,
{\rm d}z^2\,, \\
b &= \sqrt{2} {\rm e}^{h/2} \sqrt{\frac{h_1h_\be}{h_{1\b1}}} \, \,{\rm
  d}z^2\,.
\end{split}
\end{align}
{}From those, we determine the $SU(2)$ connection one--forms
\begin{align}
\begin{split}
\omega^1 &= i \frac{{\rm e}^{h/2}}{\sqrt{h_1h_\be}} (h_\be {\rm d}z^2 - h_1
{\rm d}z^\bt)\,,\\
\omega^2 &= - \frac{{\rm e}^{h/2}}{\sqrt{h_1h_\be}} (h_\be {\rm d}z^2 + h_1
{\rm d}z^\bt)\,,\\
\omega^3 &= -\frac i 2 \left(h_1 - \frac{h_{1\be}}{h_\be} +
\frac{h_{11}}{h_1} \right) {\rm d}z^1\\
&\phantom{= }-\frac i2 \left(h_2- \frac{h_{\be2}}{h_\be} +
  \frac{h_{12}}{h_1} \right) {\rm d}z^2 + c.c.\,.
\end{split}
\end{align}
As a non-trivial check, we can use the tree-level UHM metric, and these one-forms agree with the
those obtained in~\cite{Davidse:2005ef}. Notice that the situation drastically simplifies when
there is an additional killing vector in the direction $i(\partial_1 -
\partial_{\bar 1})$, because then $h_1 = h_{\bar 1}$.

We now gauge the isometry associated with $\varphi$. In the complex coordinates, this is the vector
\begin{align}
k = \frac 12 i(\partial_2 - \partial_\bt),
\end{align}
where the normalization is such that $k = \partial_\varphi$. Calculations of the moment maps is now
straight-forward and after some algebra we find
\begin{align}
\vec \mu =
\left(
  \begin{array}{l}
  \frac{{\rm e}^{h/2}} { \sqrt  {h_1 h_\be}} (h_1 + h_\be)\\
 -i \frac{{\rm e}^{h/2}} { \sqrt  {h_1 h_\be}} (h_1 - h_\be)\\
  - h_2
  \end{array}
\right),
\end{align}
which are real ($h_2 = h_\bt$).

The square of the moment maps therefore reads
\begin{align}
\vec \mu^2&= (4{\rm e}^h + h_2^2) = 4 {\rm e}^h + (\partial_\chi h)^2\,,
\end{align}
where we have used $\partial_\varphi h =0$. This last expression is valid in the coordinates
($u,\sigma,\chi,\varphi$). Changing to the coordinates ($r,\sigma,\chi,\varphi$) amounts to
changing the derivatives according to
\begin{align}
\partial_\chi \rightarrow \partial_\chi + \chi \frac{r+c}{r+2c}
\partial_r\,.
\end{align}

%%% Local Variables: 
%%% mode: latex
%%% TeX-master: "../thesis"
%%% End: 
